# Supplementary material for: Context Modeling in 3D Human Pose Estimation: A Unified Perspective
Source: arXiv:2103.15507 source file (2021-03-30)
Supplement: Supplementary file 1 [file 8supplementary.tex]

\subsection{Optimization Problem of PSM}

PSM for $3$D pose estimation \cite{PavlakosZDD17,qiu2019cross} aims to determine optimal joint locations by maximizing the following energy function with random variables $\bm{J} \in \mathcal{R}^{N \times 3}$
\begin{equation}
\begin{aligned}
\label{eq:psm_opt}
Energy(\bm{J}) = \prod_{i = 0}^{N-1} x_{i, \bm{J}_i} \prod_{(J_u, J_v) \in \mathcal{E}} \psi(\bm{J}_u, \bm{J}_v, \bm{e}_{u,v}),
\end{aligned}
\end{equation}
where $\bm{J}_u \in \mathcal{R}^{3}$ represent the $3$D position of a voxel, $x_{u,\bm{J}_u}$ is the likelihood of joint $J_u$ being at $\bm{J}_u$. The pairwise term $\psi(\bm{J}_u, \bm{J}_v, \bm{e}_{u,v})$ encodes the limb length constraints measuring whether the distance between $\bm{J}_u$ and $\bm{J}_v$ satisfies the limb length prior in $\bm{e}_{u,v}$, and is defined as 

\begin{small}
\begin{equation}
\psi(\bm{J}_u, \bm{J}_v, \bm{e}_{u,v}) =\left\{
\begin{array}{rcl}
1, & & ||\bm{J}_u - \bm{J}_v||_2 \in [\mu_{u, v} - \epsilon, \mu_{u, v} + \epsilon]\\
0, & & otherwise\\
\end{array} \right.
\end{equation}
\end{small}
in \cite{PavlakosZDD17,qiu2019cross}, where $\mu_{u, v}$ is the limb length prior encoded in $\bm{e}_{u,v}$, and $\epsilon > 0$ is a tolerance threshold.

\subsection{Reformulate GNN}
Ci \etal \cite{Ci_2019_ICCV} factor the Laplacian operator in GNN \cite{defferrard2016convolutional} into the product of a prior \emph{structure} matrix $\bm{S}$ and a learnable \emph{weight} matrix $\bm{W}$. In particular, $\bm{S}$ encodes dependence among graph nodes, according to the pre-defined human body structure. If joint $J_v$ is a contextual joint of $J_u$, then $\bm{S}^{(u, v)}$ is set to be $1$, otherwise $0$. The output features of a node $J_u$ is defined as 
\begin{equation}
\label{eq:lcn_layer}
    \bm{y}_u = \sum_{v=0}^{N-1} (\bm{S}^{(u, v)} \odot \bm{W}^{(u, v)}) \bm{x}_v,
\end{equation}
where $\bm{x}_v \in \mathcal{R}^{M_{\text{input}}}$, and $\bm{y}_u \in \mathcal{R}^{M_{\text{output}}}$. $\bm{W}^{(u, v)} \in \mathcal{R}^{M_{output} \times M_{input}}$ is the learnable weight matrix. 

\subsection{3D Network Architecture}
\begin{figure}[ht]
	\centering
	\includegraphics[width=3.2in]{imgs/v2v.pdf}
	\caption{Detailed architecture of the encoder and decoder.}
	\label{fig:v2v}
\end{figure}

\subsection{Pseudocode of TransPose}

\begin{algorithm}[htb]
    %\SetAlgoNoLine  %remove the vertical line
    % \caption{Attention-based Message Passing} 
    \caption{} 
    \label{alg:framework}
    \KwIn{$\{\bm{x}_{u,\bm{q}} \in \mathcal{R}^{M} | J_u \in \mathcal{J}, \bm{q} \in \Omega\}$ ($\bm{x}_{u,\bm{q}}$ denotes the input feature of joint $J_u$ at voxel $\bm{q}$) and known limb length priors $\{\bm{e}_{u,v} = (\mu_{u, v}, \sigma_{u, v}) | (J_u, J_v) \in \mathcal{E}\}$.}
      
    \KwOut{$\{\bm{y}_{u,\bm{q}} \in \mathcal{R}^{M} | J_u \in \mathcal{J}$, $\bm{q} \in \Omega\}$ ($\bm{y}_{u,\bm{q}}$ denotes the output feature of joint $J_u$ at voxel $\bm{q}$).}
    
    \KwParam{$\{\bm{W}_{u, v} \in \mathcal{R}^{M \times M} | J_u, J_v \in \mathcal{J}\}$ and $\{\bm{d}_v \in \mathcal{R}^{M} | J_v \in \mathcal{J}\}$.}
    
    \tcp{Compute GA for all joints}
    \For{$J_v \in \mathcal{J}$}{
        %\tcp{Normalization coefficient}
        $Z^{G}_{v} \gets \sum_{\bm{k} \in \Omega} \emph{exp}(\bm{d}^{T}_{v}\bm{x}_{v,\bm{k}})$

        \For{$\bm{k} \in \Omega$}{
            \tcp{GA $G_v(\bm{x}_{v,\bm{k}})$, Eq. \ref{eq:global}}
            $G_{v, \bm{k}} \gets \emph{exp}(\bm{d}^{T}_{v}\bm{x}_{v,\bm{k}}) / Z^{G}_{v}$
        }
    }    
    \tcp{Message passing between joints}
    \For{$J_u \in \mathcal{J}$}{
      \For{$\bm{q} \in \Omega$}{
        \For{$J_v \in \mathcal{N}_u$}{
          %\tcp{Normalization coefficient}
          $Z^{P}_{u, v, \bm{q}} \gets \sum_{\bm{k} \in \Omega} A^{g}_{v, \bm{k}}\emph{exp}(- \frac{ (||\bm{q}-\bm{k}||_2-\mu_{u,v})^2}{2\alpha\sigma_{u,v}^2 + \epsilon})$
          
          \For{$\bm{k} \in \Omega$}{                  
            \tcp{PA $P(\bm{q},\bm{k}, \bm{e}_{u,v}$), Eq. \ref{eq:pairwise}}
            $P_{u,v,\bm{q},\bm{k}} \gets \emph{exp}(- \frac{ (||\bm{q}-\bm{k}||_2-\mu_{u,v})^2}{2\alpha\sigma_{u,v}^2 + \epsilon}) / Z^{P}_{u,v, \bm{q}}$
          }
        }
        \tcp{Update $\bm{y}_{u,\bm{q}}$, Eq. \ref{eq:transpose_general}} 
        % $\bm{y}_{u,\bm{q}} \gets \bm{x}_{u,\bm{q}} + \sum_{J_v \notin \mathcal{N}_u} \sum_{\bm{k} \in \Omega} A_{v, \bm{k}}^{g} \cdot \bm{W}_{u, v} \bm{x}_{v,\bm{k}} + \sum_{J_v \in \mathcal{N}_u} \sum_{\bm{k} \in \Omega} A_{v, \bm{k}}^{g} \cdot A_{u,v, \bm{q},\bm{k}}^{p} \cdot \bm{W}_{u, v} \bm{x}_{v,\bm{k}}$
        $\bm{y}_{u,\bm{q}} \gets \bm{x}_{u,\bm{q}} + \sum_{J_v \in \mathcal{J}} \sum_{\bm{k} \in \Omega} G_{v, \bm{k}} \cdot P_{u,v, \bm{q},\bm{k}} \cdot \bm{W}_{u, v} \bm{x}_{v,\bm{k}}$
      }
    }
\end{algorithm}
